# Supplementary material for: Generalised Mutual Information: a Framework for Discriminative Clustering
Source: arXiv:2309.02858 source file (2023-09-06)
Supplement: Supplementary file 1 [file gemini_gradients.tex]

\section{Gradients of \texorpdfstring{$f$}{f}-divergence GEMINIs}

We will show in this section the derivations of the gradient $\nabla$ w.r.t. the parameters $\theta$ of the posterior distribution $\pyx$ for the $f$-divergence GEMINIs. Note that the discrete variable $y$ for the cluster assignment has a distribution depending on the parameters $\theta$ whereas the $\pdata$ distribution does not.

\subsection{OvA \texorpdfstring{$f$}{f}-divergences}

For any f-divergence, we can rewrite the one-vs-all GEMINI by extending the expectation over the discrete cluster assignments:

\begin{equation*}
    \mathcal{I}^\text{ova}_\text{f-div} = \E_{\pdata,\py} \left[ f\left( \frac{\pyx}{\py}\right)\right] = \E_{\pdata} \left[ \sum_{y=1}^K \py f \left( \frac{\pyx}{\py} \right)\right]\quad.
\end{equation*}

We can now start applying the gradient operator $\nabla_\theta$:

\begin{equation*}
    \nabla_\theta \mathcal{I}_\text{f-div}^\text{ova} = \nabla_\theta \E_{\pdata} \left[ \sum_{y=1}^K \py f\left( \frac{\pyx}{\py}\right)\right]\quad.
\end{equation*}

First, as the data distribution $\pdata$ is constant w.r.t. the parameters $\theta$, we can perform the derivation inside the expectation:

\begin{align*}
    \nabla_\theta \mathcal{I}_\text{f-div}^\text{ova} &= \E_{\pdata} \left[ \nabla_\theta \sum_{y=1}^K \py f\left( \frac{\pyx}{\py}\right)\right]\\
    &= \E_{\pdata} \left[ \sum_{y=1}^K \py \nabla_\theta f\left( \frac{\pyx}{\py}\right) + f\left( \frac{\pyx}{\py}\right) \nabla_\theta \py\right]\quad.
\end{align*}

We unfold the derivatives:

\begin{align*}
    \nabla_\theta \mathcal{I}_\text{f-div}^\text{ova} &= \E_{\pdata} \left[ \sum_{k=1}^K \py f^\prime \left(\frac{\pyx}{\py}\right) \nabla_\theta \frac{\pyx}{\py} + f\left(\frac{\pyx}{\py}\right)\nabla_\theta \py\right]\\
    &= \E_{\pdata} \left[ \sum_{k=1}^K \py f^\prime \left(\frac{\pyx}{\py}\right) \frac{\py\nabla_\theta \pyx - \pyx \nabla_\theta \py}{\py^2} \right.\\&\qquad\left.+ f\left(\frac{\pyx}{\py}\right)\nabla_\theta \py \right]\\
    &= \E_{\pdata} \left[ \sum_{k=1}^K f^\prime \left(\frac{\pyx}{\py}\right)\nabla_\theta \pyx \right.\\&\qquad\left.+ \left\{f\left(\frac{\pyx}{\py}\right) - \frac{\pyx}{\py}f^\prime \left(\frac{\pyx}{\py}\right)\right\}\nabla_\theta \py \right]\quad.
\end{align*}

However, the marginal is estimated directly as the expectation of the posterior over the data. In practice, we use an unbiased estimate for the marginal. Therefore, the gradient of the marginal w.r.t $\theta$ becomes:

\begin{equation*}
\nabla_\theta \py = \E_{\pdata} [\nabla_\theta \pyx]\quad,
\end{equation*}

which we can re-inject in the equation above:

\begin{align*}
    \nabla_\theta \mathcal{I}_\text{f-div}^\text{ova} &= \E_{\pdata} \left[ \sum_{k=1}^K f^\prime \left(\frac{\pyx}{\py}\right)\nabla_\theta \pyx \right.\\&\qquad\left.+ \left\{f\left(\frac{\pyx}{\py}\right) - \frac{\pyx}{\py}f^\prime \left(\frac{\pyx}{\py}\right)\right\}\E_{p_\text{data}(\vec{x}^\prime)} [\nabla_\theta \p(y|\vec{x}^\prime)] \right]\quad.
\end{align*}

We then realize that since $\vec{x}$ and $\vec{x}^\prime$ are drawn from the same distribution, it is equivalent to rearrange the equation thanks to expectations' linearity in order to factor everything by the same posterior gradient $\nabla_\theta \pyx$:

\begin{align*}
    \nabla_\theta \mathcal{I}_\text{f-div}^\text{ova} &= \E_{\pdata} \left[ \sum_{k=1}^K \left\{f^\prime \left(\frac{\pyx}{\py}\right) + \E_{p_\text{data}(\vec{x}^\prime)}\left[f\left(\frac{\p(y|\vec{x}^\prime)}{\py}\right) - \frac{\p(y|\vec{x}^\prime)}{\py}f^\prime \left(\frac{\p(y|\vec{x}^\prime)}{\py}\right)\right] \right\} \nabla_\theta \pyx\right]\\
    &= \E_{\pdata,\py} \left[ \frac{1}{\py}\left\{f^\prime \left(\frac{\pyx}{\py}\right) \right.\right.\\&\left.\left.\qquad+ \E_{p_\text{data}(\vec{x}^\prime)}\left[f\left(\frac{\p(y|\vec{x}^\prime)}{\py}\right) - \frac{\p(y|\vec{x}^\prime)}{\py}f^\prime \left(\frac{\p(y|\vec{x}^\prime)}{\py}\right)\right] \right\} \nabla_\theta \pyx\right]\quad.\\
\end{align*}

Therefore the gradient of the OvA $f$-divergence-GEMINI consists in two terms. The first one depends on both the value of the data $\vec{x}$ and the cluster assignment $y$, whereas the second only depends on the cluster assignment $y$ since it consists in an expectation over the data.

\subsection{OvO \texorpdfstring{$f$}{f}-divergences}

%For the \gls{ovo} $f$-divergence GEMINI, we first need to write the following useful derivative:

%\begin{equation*}
%\nabla_\theta \pxy = \pdata \nabla_\theta \frac{\pyx}{\py} = \pdata \left(\frac{\nabla_\theta \pyx}{\py} - \frac{\pyx}{\py^2}\nabla_\theta \py\right)\quad.
%\end{equation*}

Once again, the data distribution does not undergo the gradient operator for it does not depend on the parameters $\theta$. Next, we pass the gradient operator inside the data expectation.

\begin{align*}
    \nabla_\theta \mathcal{I}^\text{ovo}_\text{f-div} &= \nabla_\theta \E_{\pya,\pyb,\pdata} \left[ \frac{\pyxb}{\pyb}f\left(\frac{\pyxa\pyb}{\pyxb\pya}\right)\right]\\
    &= \E_{\pdata} \left[ \sum_{\substack{\ya=1\\\yb=1}}^{K,K} \nabla_\theta \pya \pyxb f\left(\frac{\pyxa\pyb}{\pyxb\pya}\right)\right]\quad.
\end{align*}

For concision, we will note the inner fraction:

\[\gamma = \frac{\pxya}{\pxyb} =\frac{\pyxa\pyb}{\pyxb\pya}\quad,\]

which derivative w.r.t. $\theta$ is:

%\begin{align*}
%\nabla_\theta \gamma &= \frac{\pyxb\pya \nabla_\theta \left( \pyxa\pyb\right) - \pyxa\pyb \nabla_\theta \left(\pyxb\pya \right)}{\left(\pyxb\pya\right)^2}\\
%&= \frac{\pyxb\pya \left(\pyxa\nabla_\theta \pyb + \pyb \nabla_\theta \pyxa \right)}{\left(\pyxb\pya\right)^2} \\&\quad - \frac{\pyxa\pyb \left(\pya \nabla_\theta \pyxb + \pyxb \nabla_\theta \pya \right)}{\left(\pyxb\pya\right)^2}\quad.
%\end{align*}

%Notice that we can simplify further the notation of the derivative of $\gamma$ by replacing most of the fractions with $\gamma$ itself:

\begin{equation*}\nabla_\theta \gamma = \frac{\gamma}{\pyb} \nabla_\theta \pyb + \frac{\gamma}{\pyxa} \nabla_\theta \pyxa - \frac{\gamma}{\pyxb}\nabla_\theta \pyxb - \frac{\gamma}{\pya} \nabla_\theta \pya\quad.\end{equation*}

We can now inject these elements inside the main derivative:

\begin{align*}
    \nabla_\theta \mathcal{I}^\text{ovo}_\text{f-div}&= \E_{\pdata} \left[ \sum_{\substack{\ya=1\\\yb=1}}^{K,K} \nabla_\theta \pya \pyxb f(\gamma)\right] \\
    &= \E_{\pdata} \left[ \sum_{\substack{\ya=1\\\yb=1}}^{K,K} \pyxb f(\gamma) \nabla_\theta \pya + \pya f(\gamma) \nabla_\theta \pyxb + \pya \pyxb f^\prime (\gamma) \nabla_\theta \gamma\right]\quad. \\
\end{align*}

We detail the derivation of the last term inside the expectation by first noticing that the front factor can be rewritten with the inverse of $\gamma$, then develop and simplify the fractions:

\begin{align*}
    \pya\pyxb f^\prime(\gamma)\nabla_\theta \gamma &= \frac{\pyxa\pyb}{\gamma} f^\prime(\gamma) \nabla_\theta \gamma\\
    &= \frac{\pyxa\pyb}{\gamma} f^\prime(\gamma) \left(\frac{\gamma}{\pyb} \nabla_\theta \pyb + \frac{\gamma}{\pyxa} \nabla_\theta \pyxa \right.\\&\qquad\left.- \frac{\gamma}{\pyxb}\nabla_\theta \pyxb - \frac{\gamma}{\pya} \nabla_\theta \pya \right)\\
    &=f^\prime(\gamma) \left( \pyxa \nabla_\theta \pyb + \pyb \nabla_\theta \pyxa - \pya \gamma \nabla_\theta \pyxb \right.\\&\qquad\left.- \pyxb \gamma \nabla_\theta \pya\right)\quad.
\end{align*}

We can now rewrite all inner terms of the expectation factorised with their respective gradient term:

\begin{align*}
    \nabla_\theta \mathcal{I}^\text{ovo}_\text{f-div}&= \E_{\pdata} \left[ \sum_{\substack{\ya=1\\\yb=1}}^{K,K}  \left( f(\gamma) - \gamma f^\prime(\gamma) \right) \pyxb \nabla_\theta \pya + \pyxa f^\prime(\gamma) \nabla_\theta \pyb\right.\\&\qquad\left.\vphantom{\sum_{\substack{\ya=1\\\yb=1}}^{K,K}} + \pyb f^\prime(\gamma) \nabla_\theta \pyxa + \left(f(\gamma) - \gamma f^\prime(\gamma) \right) \pya \nabla_\theta \pyxb\right]\quad. \\
\end{align*}

Since the two random variables $\ya$ and $\yb$ are in the same space and independent, all terms have a symmetric version which simply consists in swapping the position of the index $a$ or $b$. Note that the swapped version of $\gamma$ is $1/\gamma$. We can therefore write a new version of the gradient that only depends on the gradient of the marginal and posterior of one single cluster assignment $\ya$:

\begin{align*}
    \nabla_\theta \mathcal{I}^\text{ovo}_\text{f-div}&= \E_{\pdata} \left[ \sum_{\ya=1}^K \left\{ \sum_{\yb=1}^K \pyxb\left(f(\gamma) -f^\prime(\gamma) + f^\prime(\frac{1}{\gamma}) \right) \nabla_\theta \pya \right.\right.\\
    &\quad\left.\left. \sum_{\yb=1}^K \pyb \left( f(\frac{1}{\gamma}) - \frac{1}{\gamma}f^\prime(\frac{1}{\gamma}) + f^\prime(\gamma)\right)\nabla_\theta \pyxa \right\}\right]\quad.
\end{align*}

We can now introduce the function $h$ defined as:

\begin{equation*}
    h(t) = f(t) -t f^\prime(t) +f^\prime(\frac{1}{t})\quad,
\end{equation*}

which we can recognize in our gradient and thus simplify the notation:

\begin{equation*}
    \nabla_\theta \mathcal{I}^\text{ovo}_\text{f-div} = \E_{\pdata} \left[ \sum_{\ya=1}^K \sum_{\yb=1}^K \pyxb h(\gamma) \nabla_\theta \pya + \sum_{\yb=1}^K \pyb h(\frac{1}{\gamma}) \nabla_\theta \pyxa\right]\quad.
\end{equation*}

We finish this step by replacing sums in the equation by expectations:

\begin{equation*}
\nabla_\theta \mathcal{I}^\text{ovo}_\text{f-div} = \E_{\pdata, \pya} \left[ \frac{1}{\pya} \E_{\pyb}\left[\frac{\pyxb}{\pyb}h(\gamma)\right]\nabla_\theta \pya +\frac{1}{\pya}\E_{\pyb} \left[h(\frac{1}{\gamma}) \right]\nabla_\theta \pyxa\right]\quad.
\end{equation*}

In order to finish this demonstration, we perform the same trick as in the OvA scenario. In practice, the cluster proportion are estimated via the posterior distribution, and so must we unfold the expression $\nabla_\theta \pya$:

\begin{equation*}
    \nabla_\theta \pya = \nabla_\theta \E_{\pdata} \left[ \pyxa \right] = \E_{\pdata} \left[ \nabla_\theta \pyxa \right]\quad,
\end{equation*}

leading to:

\begin{equation*}
    \nabla_\theta \mathcal{I}^\text{ovo}_\text{f-div} = \E_{\pdata, \pya} \left[ \frac{1}{\pya} \E_{\pyb}\left[\frac{\pyxb}{\pyb}h(\gamma)\right] \times \E_{p_\text{data}(\vec{x}^\prime)} \left[ \nabla_\theta \p(\ya|\vec{x}^\prime)\right] +\frac{1}{\pya}\E_{\pyb} \left[h(\frac{1}{\gamma}) \right]\nabla_\theta \pyxa\right]\quad.
\end{equation*}

Then, we can reorder the elements thanks to the linearity of the expectation:

\begin{equation*}
    \nabla_\theta \mathcal{I}^\text{ovo}_\text{f-div} = \E_{\pdata, \pya} \left[ \frac{1}{\pya} \E_{\pyb} \left[ h(\frac{1}{\gamma}) - \E_{p_\text{data}(\vec{x}^\prime)}\left[\frac{\p(\yb|\vec{x}^\prime)}{\pyb} h(\gamma) \right] \right]\nabla_\theta \pyxa\right]\quad.
\end{equation*}

For the final equation, we can expand again the definition of $\gamma$:

\begin{equation*}
    \nabla_\theta \mathcal{I}^\text{ovo}_\text{f-div} = \E_{\pdata, \pya} \left[ \frac{1}{\pya} \E_{\pyb} \left[ h \left(\frac{\pxyb}{\pxya}\right) - \E_{p_\text{data}(\vec{x}^\prime)}\left[\frac{\p(\yb|\vec{x}^\prime)}{\pyb} h\left(\frac{\p(\vec{x}^\prime|\ya)}{\p(\vec{x}^\prime|\yb)}\right) \right] \right]\nabla_\theta \pyxa\right]\quad.
\end{equation*}

Thus, we highlighted for both the OvA and OvO GEMINIs based on $f$-divergences that gradients consists in two terms within an expectation. The first one varies both with the values of the cluster assignment $y$ and the data sample $\vec{x}$, whereas the second one only varies with $y$.
